# Supplementary material for: Query Rewriting On Path Views Without Integrity Constraints
Source: arXiv:2010.03527 source file (2020-10-07)
Supplement: Supplementary file 1 [file weak_plans.tex]

\subsection{Characterising Weakly Smart Plans}

In this section, we are interested in characterising weakly smart plan. We already know that all smart plans are also weak, so the previous section give a partial characterisation. We will see that we can complete it by introducing \textit{loosely bounded plans}. These new plans look like reversed bounded plans: We first cross the query  and then perform a forward path followed by a walk. The idea is that some results might be filtered due to the forward path but, at the end, if we get a result, it means some answers had to survive.

\begin{Definition}[Loosely Bounded Plan]\label{loosely-bounded-plan}
A loosely bounded path for a set of relations $\mathcal{R}$ and a query $q(x) \leftarrow r(a, x)$ is either a bounded path or a path query of the form $r.P.B$, where $r.P$ is a path query, and $B$ is a walk through $r^-.P$ to the position $1$.

A loosely bounded plan for a set of functions $\mathcal{F}$ is an non-redundant execution plan whose consequences are a loosely bounded path.
\end{Definition}

\noindent The difference to bounded plans (Definition~\ref{def:bounded-plan}) is thus that the query can also appear at the beginning of the path. As we did for smart plans, we are now going to show the correctness and the completeness of the loosely bounded plans.

\begin{Theorem}[Correctness]\label{thm:loosely-bounded-correct}
    Let $q(x) \leftarrow r(a, x)$ be an atomic query, $F$ a set of path functions and $F_{sub}$ the set of sub-functions of $F$. Let $\pi_a$ be a non-redundant loosely bounded execution plan over the $F_{sub}$. Then $\pi_a$ is weakly smart.
\end{Theorem}

\begin{proof}
Let us first prove that every loosely bounded plan is weakly smart.
If the loosely bounded plan is a bounded plan (Definition~\ref{def:bounded-plan}), then it is a smart plan (Theorem~\ref{thm:bounded-correct}). Hence, it is also a weakly smart plan.
Let us now consider the plans of the form $\pi_a=r.P.B$, where $r.P$ is a path query, and $B$ is a walk through $r^-.P$ to the position $1$. Take any database $\mathcal{I}$ such that $q(I) \neq \emptyset$ and $\pi_a(I) \neq \emptyset$. Let $\mathcal{C} = q(I)$.
Let use write $\pi_a(x)=r.P.B(a, x)=r(a, x_1).r_1(x_1, x_2)...r_n(x_n, x_{n+1}).B(x_{n+1}, x)$. Let $\sigma$ be a binding of the variables of $\pi_a$ in $\mathcal{I}$. We know such binding exists as $\pi_a(I) \neq \emptyset$. Let $c = \sigma(x_1)$. We know that $c \in \mathcal{C}$ as the first relation is $r$. Using the same arguments as in Theorem~\ref{thm:bounded-correct}, we can show that $c \in P.B(c)$. Thus, $c \in r.P.B(a)$ and so the plan is weakly smart.
\end{proof}

\begin{Theorem}[Completeness]\label{thm:loosely-bounded-complete}
    Let $q(x) \leftarrow r(a, x)$ be an atomic query, $F$ a set of path functions and $F_{sub}$ the set of sub-functions of $F$. Let $\pi_a$ be a weakly smart plan over the $F_{sub}$. Then $\pi_a$ is loosely bounded.
\end{Theorem}

\begin{proof}
Let $\pi_a$ be a weakly smart plan for a query $q(x) \leftarrow r(a, x)$, with consequences $r_1(x_1,x_2)...$ $r_n(x_n,x_{n+1})$. For convenience, we write $a = c_1$
Consider the database $\mathcal{I}$:
	\[\mathcal{I}=\{r^-(c_0,c_1), r_1(c_1,c_2), ..., r_n(c_n,c_{n+1})\}\]
Here, the $c_i$ are fresh constants.
Let us first assume that $r_1 \neq r$. Then, $\pi_a(\mathcal{I}) \supseteq \{c_{n+1}\} \neq \emptyset$ and $q(\mathcal{I})=\{c_0\}$. Since $\pi_a$ is weakly smart, we must have $c_0 \in \pi_a(\mathcal{I})$. Using the same argument as in Theorem~\ref{thm:bounded-complete}, $\pi_a$ must be a forward path $P$, followed by a walk $B$ in $r^-P$. Hence, $\pi_a$ is a bounded plan.

Let us now suppose that $r_1 = r$. We now have $q(\mathcal{I})=\{c_0, c_2\}$. Since $\pi_a$ is weakly smart, we must have $c_0 \in \pi_a(\mathcal{I})$ or $c_2 \in \pi_a(\mathcal{I})$ (or both). Let us consider the first case. Using the same argument as before, $\pi_a$ must consist of a forward path $P$ followed by a walk $B$ in $r^-.P$. That is, $\pi_a$ is a bounded plan. In that case, $\pi_a(\mathcal{I})=\{c_0, c_2\}$, and $\pi_a$ is actually a smart plan.

Now consider the case where $c_2 \in \pi_a(\mathcal{I})$ and $c_0 \not\in \pi_a(\mathcal{I})$. We can then proceed the same way we did in Theorem~\ref{thm:bounded-complete}. We take the same notations, with a binding such that $\sigma(x_{n+2}) = c_2$. We call $r_1...r_m = r.r_2...r_m$ the \textit{forward path}. The induction then proceeds the same way. The only difference is that we have to stop at position $1$ as we must end on $c_2$.
\end{proof}

We see here that smart plans and weakly smart plan are different. Let us consider the following example to better understand why it is the case.

\begin{Example}
We continue with the music example. We have access to two path functions: $getAlbumsOfSinger(singer, album) = sing(singer, song), onAlbum(song,$ $album)$ which gets all the albums on which a singer sings and $getSongsOnAlbum(album,$ $song) = onAlbum^-(album,$ $song)$ which gives us the songs on an album. Our query is $q_{Pomme}(x) = sing(Pomme, x)$. The plan $\pi_{Pomme}(x) = getAlbumsOfSinger(Pomme,$ $album), getSongsOnAlbum(album, x)$ is weakly smart but not smart. Indeed, if we consider the database $mathcal{I} = \{sing(Pomme, Pauline), sing(Pomme,$ Itsumo Nando Demo$), onAlbum(Pauline,$ À peu près$)\}$, then the plans return $Pauline$ but not \textit{Itsumo Nando Demo}, which was never published on an album.
\end{Example}
